# Supplementary material for: Chemical and Crystallographic Characterization of the Tip Apex in Scanning Probe Microscopy
Source: arXiv:1310.6574 source file (2014-02-12)
Supplement: Supplementary file 1 [file Supplemental_Information.pdf]

# Supplemental Information

## Chemical and Crystallographic Characterization of the Tip Apex in Scanning Probe Microscopy

Thomas Hofmann, Florian Pielmeier, and Franz J. Giessibl
Institute of Experimental and Applied Physics, University of Regensburg, D-93053 Regensburg, Germany

## S 1 Modification and characterization of the tip apex

Prior to the measurements on the CO/Cu(111) sample, the tips of the force sensors were inserted in the field ion microscope that is part of the ultrahigh vacuum system which also contains the low temperature scanning tunneling/atomic force microscope (LT STM/AFM). Tips were cleaned by field evaporation with a voltage of up to 15 kV and transferred *in situ* to the LT STM/AFM. This is a standard procedure for cleaning tips in a field ion microscope [1] and allows for complete removal of the native oxide layer. Stable tunneling was observed with all tips directly after the approach to the Cu(111) surface.

During the characterization measurements the tip apex was modified by poking it into the Cu surface. We distinguish two kinds of pokes. Indenting the tip several nanometers into the metallic sample surface is defined as a strong poke. This is a standard procedure within the low temperature scanning tunneling microscopy community to prepare stable and reliable tips [2–4]. Strong pokes lead to craters in the sample surface with a depth of several nanometers. The result of a strong poke on the Cu surface is shown in Fig. S 1. In this example, the tip was approached 20 nm towards the surface. It has been assumed within the low temperature STM community that strong pokes in soft metals such as Cu lead to a wetting of the tip by sample material [5]. Indeed, we could confirm that W tips are usually covered by Cu after performing strong pokes on a Cu sample by the tip identification methods outlined in this manuscript.

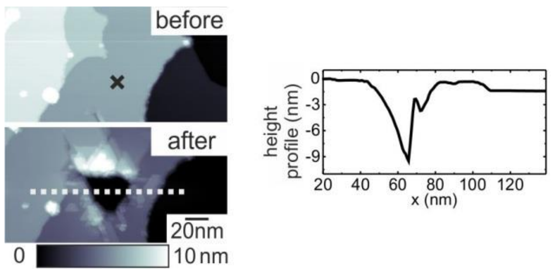


Fig. S 1 STM overview images before and after a strong poke. The poke involved a 20 nm advance of the tip towards the sample at the position marked by an ‘x’. The height profile through the minimum of the poke site on the right (its trace is shown as a dotted line in the left bottom image) reveals that the strong poke resulted in a crater with a depth of almost 10 nm.

In contrast to strong pokes, gentle pokes can merely lead to recrystallizations of the front-most part of the tip apex without a material transfer from sample to tip or vice versa [6]. For a gentle poke, the tip is positioned above the clean Cu surface in STM feedback (current setpoint: 100 pA, bias: -10 mV). The corresponding tunneling resistance of 100 MΩ (a conductance of 10 nS) corresponds to a distance of about 420 pm from point contact over the Cu

surface (see section S 2), where the quantum point contact resistance of 12.9 kΩ holds. The tip is approached between 400 to 900 pm and then retracted while a bias voltage between 0.5 and 5 V is applied. Before and after each gentle poke, a STM overview image is recorded. Additionally, the tip apex is characterized by COFI before and after each poke. Fig. S 2 a illustrates the sequence of characterizing and manipulating the tip apex. The details of COFI images are given in section S 2.

Fig. S 2 b-d schematically illustrates the three possible effects of gentle pokes on the sample surface and on the tip apices. The STM overview images before and after reveal the effects of the pokes on the sample surface. The poke sites are indicated by an 'x'. It is important to note that usually the STM images do not change significantly after pokes; however, the COFI images that show the force channel clearly reflect how the poke changed the tip apex.

The example in Fig. S 2 b represents the most common result of a gentle poke, i.e. one or several small bumps on the surface. These consist of single or multiple atoms which have been deposited from the tip. In Fig. S 2 b, the COFI image of the tip apex has changed from a twofold to a toroidal symmetry, indicating that the orientation of the tip cluster has changed. Generally, it is assumed that atoms released from the tip are surface atoms which were picked up beforehand during tip

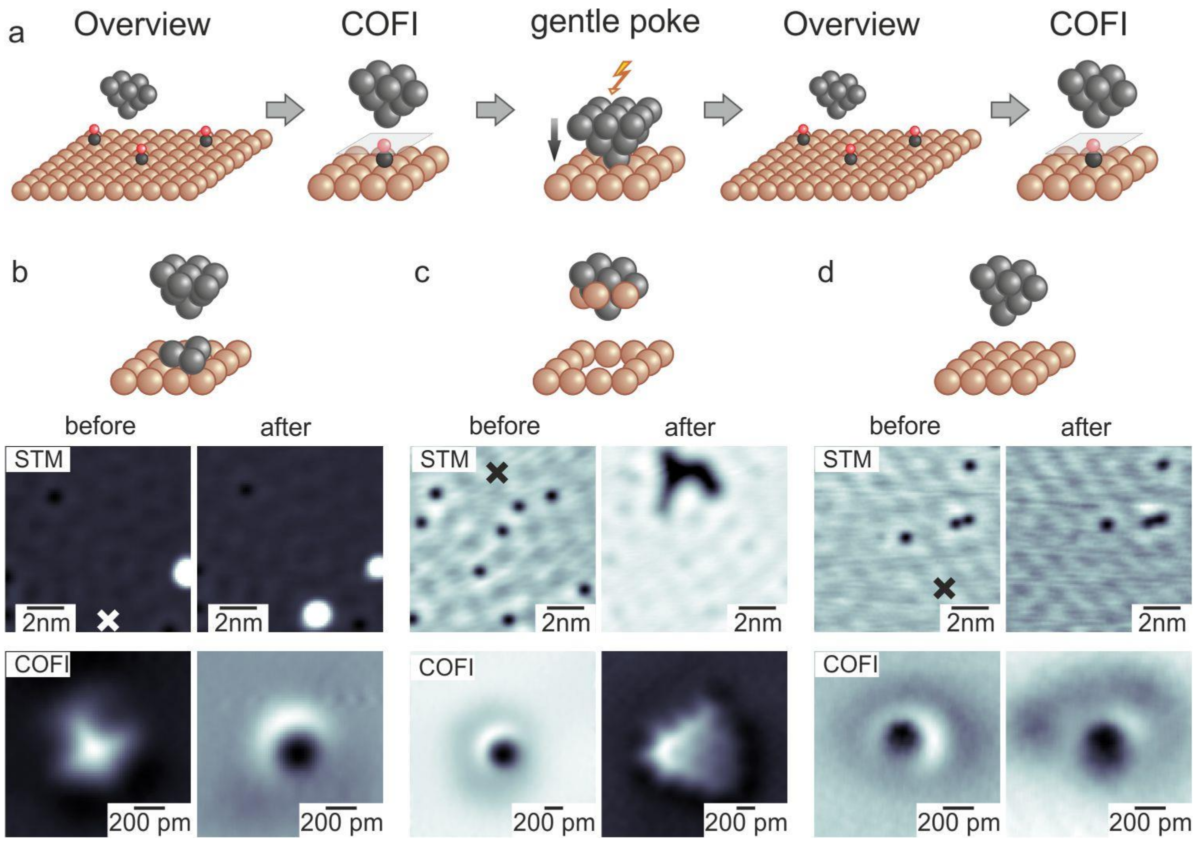


Fig. S 2 a) Sequence of a typical measurement: Before and after each poke, a STM overview image (10×10 nm$^2$) and a COFI image are recorded. The overview image reveals the effect of the poke on the sample surface. A change of the tip cluster is identified by the COFI images. The pokes can result in a bump (b) or a void (c) on the surface. In rare cases, the surface is not affected by the poke (d), although the tip cluster has changed. The bump in the before image in (b) originates from a previous poke. The COFI image after the poke in (c) shows a tip cluster that is terminated by a small, triangular terrace (see description in the text). Note that the area of the COFI images is 2×2 nm$^2$ in (c), in contrast to 1.5×1.5 nm$^2$ in (b) and (d).

preparation by indentation [2,3,5]. But it is also possible that the bumps consist of atoms from the tip material.

Fig. S 2 c shows that a poke can also lead to a void in the surface. In this case Cu atoms are transferred from the sample to the tip. Before poking, the COFI image showed a toroidal tip image. Afterwards the COFI image revealed a triangle whose size is larger than the tip image of a single atom tip. A hexagonal lattice with six minima is visible within the triangle indicating that the tip is terminated by a triangular terrace of about six atoms. The atomic spacing is close to the nearest neighbor distance in Cu ($d_{NN}$ = 255 pm), and the void created by the poke suggests that the tip-terminating triangular terrace consists of Cu. As the bulk tip material was W in this example, the Cu atoms at the tip apex were picked up from the surface. However, in general the adsorbed atoms must not necessarily end up at the tip apex but might also diffuse to the side of the tip.

In rare cases, gentle pokes alter the tip cluster without affecting the sample surface, i.e. neither is sample material picked up from the tip, nor are atoms originating from the tip dropped to the surface (see Fig. S 2 d or the tips 1, 2 and 3 presented in Ref. [6]). The STM overview image before and after the poke shows neither a protrusion nor a depression. However, the apparent depth of the CO molecules is different in the two images and the two neighboring CO molecules are resolved more clearly in the image recorded before the poke. These observations already suggest that the tip cluster has changed. The COFI images support this claim, as they show two different circular symmetric tips.

## S 2 Acquisition and analysis of the COFI images and force versus distance curves

In FM-AFM, the key observable is the frequency shift $\Delta f$ which directly corresponds to an averaged force gradient $\langle k_{ts} \rangle = \Delta f/f_0 \times 2k$. This allows to compare the physics of measurements (average force gradients) obtained with sensors that have alternate resonance frequencies $f_0$ and stiffnesses $k$. In the following table, the parameters of all sensors ($f_0$, $k$ and the quality factor $Q$) are shown:

| Measurement type | $k$ (N/m) | $f_0$ (Hz) | $Q$ |
|---|---|---|---|
| All Cu tips | 1800 | 26968.8 | 134705 |
| Fe<100>-1 | 1800 | 59368.9 | 355500 |
| Fe<100>-2 | 1800 | 23899.7 | 27280 |
| Fe<110>-1 | 1800 | 28030.8 | 22025 |
| Fe<110>-2 | 1800 | 59369.4 | 1120100 |
| Fe<111>-1 | 1800 | 28030.9 | 20500 |
| W<100>-1 | 1800 | 27845.7 | 28305 |
| W<111>-1 | 1800 | 27846.6 | 28305 |

In addition to the force gradient $\langle k_{ts} \rangle$, the tunneling current is collected simultaneously. As the tip oscillates the tunneling current is averaged over several oscillation cycles. The sample voltage was set to -10 mV in all measurements.

The COFI image is the $\langle k_{ts} \rangle$ map that is recorded in constant height (CH) mode at a tip-sample distance close to the manipulation distance. This distance is determined experimentally by reducing the tip-sample distance in 10 pm steps until the CO is manipulated during imaging. At the distance of the COFI image the averaged tunneling current above the bare Cu surface is between 15 to 25 nA,

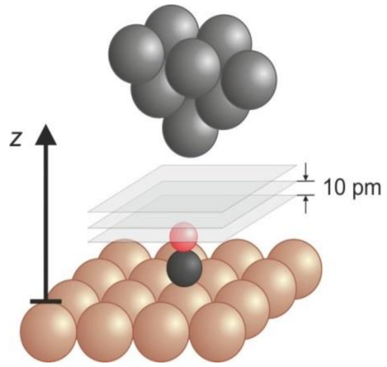


Fig. S 3 Acquisition of the constant height maps for the 3D force spectroscopy

corresponding to an average gap resistance of 333 to 400 kΩ. The COFI images only display the short range force components. The long range forces are subtracted. For this purpose, an averaged $\langle k_{ts} \rangle$ value is determined over the Cu surface. As we do not observe atomic resolution on the Cu surface, this value is attributed to long-range forces and therefore subtracted as a long range background from all image data, as proposed in Ref. [7].

The force distance curves are obtained either from a three-dimensional $\langle k_{ts} \rangle$ dataset or from point spectroscopy. For the 3D $\langle k_{ts} \rangle$ dataset, multiple CH maps are recorded by subsequently increasing the tip-sample distance in increments of 10 pm, starting with the closest distance where the COFI image was taken. The distance is increased until the contrast difference between Cu and CO vanishes completely, typically at a height increase of about 0.5 nm. Hence, we usually record 50 maps and each map takes about 8 min. This sums up to a total of about 6.5 h acquisition time for a three dimensional data set. During this time, the feedback is switched off and the system is subject to thermal drift and piezo creep. The drift in the *x*- and *y*-directions is corrected by cross-correlating the current images over the whole distance range. The drift in *z*-direction is corrected with the help of fast current versus distance curves. These curves are acquired by point spectroscopy before or after the maps over the clean Cu surface at a fast speed where creep and drift are negligible. The curves are fitted by an exponential function with a decay constant $\kappa$, yielding a precise current versus height reference. The decay constant is used to determine the tip-sample distance from the tunneling current for each map, as explained in detail in section S 3. As in the case of the COFI image, the contribution of long range forces is subtracted in each $\langle k_{ts} \rangle$ map. Afterwards the 3D $\langle k_{ts} \rangle$ data set is deconvolved with the help of the Sader-Jarvis method [8] to obtain the 3D data set of the short range forces.

The point spectroscopy is acquired by retracting the tip by a distance of 800 pm with a velocity of 25 pm/s while $\langle k_{ts} \rangle(z)$ is recorded. For <100> tips, the minima in the $\langle k_{ts} \rangle(z)$ curves can only be observed by point spectroscopy. The reason is that the lateral forces exceed the manipulation threshold when moving the tip over the CO molecule at the distance where the vertical force minimum occurs. In addition to each point spectrum recorded over CO, a complementary one is recorded over the Cu surface. The $\langle k_{ts} \rangle(z)$ curve over Cu is subtracted from the one recorded over the CO molecule to remove the contribution of the long range forces. The resulting $\langle k_{ts} \rangle(z)$ curve is deconvolved by the method of Sader and Jarvis [8] to determine the force distance curve.

## S 3 Determination of the tip-sample distance

If we assume that the tunneling current is dominated by a single apex atom, we can reference the tip-sample distance *z* at the lower turnaround point of the oscillation to quantum point contact with the conductivity $G_0 = 2e^2/\hbar$ with the help of the following equation [6]:

$$z = \frac{1}{2\kappa} \ln\left( \frac{\langle I(z) \rangle}{I_0^{\text{Bessel}}(2\kappa A) \cdot G_0 \cdot V_{sample}} \right) - A\,, \qquad (1)$$

with the Bessel function of order zero $I_0^{\text{Bessel}}(2\kappa A)$ and the current decay constant $\kappa$. The Bessel function is used to calculate the maximum tunneling current at the lower turnaround point from $\langle I(z) \rangle$, which is averaged over the oscillation cycle. The decay constant $\kappa$ is determined from current point spectra by fitting an exponential decay to the current versus distance curve. We obtain values between 9.6 nm$^{-1}$ and 10 nm$^{-1}$, which are typical for metal-metal tunneling gaps.

However, we found that $\langle k_{ts} \rangle(z)$ curves of tips with the same orientation can be offset by values as great as 50 pm. The reason is that the tunneling current does not only originate from the front atom but also contributions from atoms of the second tip layer are measured. As an effect, blunt tips yield a larger current compared to sharp tips if both are held at the same front-atom to sample distance. The sharpness of the tip can be estimated by the apparent depth of the CO molecule (Fig. S 4 a), measured at a moderate tip-sample distance – e.g. $I_{set}$ = 100 pA, $V_{sample}$ = -10 mV – to avoid an influence of the forces between the tip atom and the CO molecule. Evaluating all measurements, we found a maximum depth $C_{sharp}$ = 43 pm. This value is taken as a reference for correcting the tip-sample distance in the force versus distance curves, which were obtained with tips which show a smaller apparent depth $C_{blunt}$. Assuming that the decay constant has the same value over CO and over the Cu(111) surface, we can renormalize the current measured with a blunt tip $I_{blunt}$ with the help of the difference in the observed apparent depth $\Delta C = C_{blunt} - C_{sharp}$:

$$I_{blunt} = I_{sharp} \times \exp(-2\kappa\Delta C) \qquad (2)$$

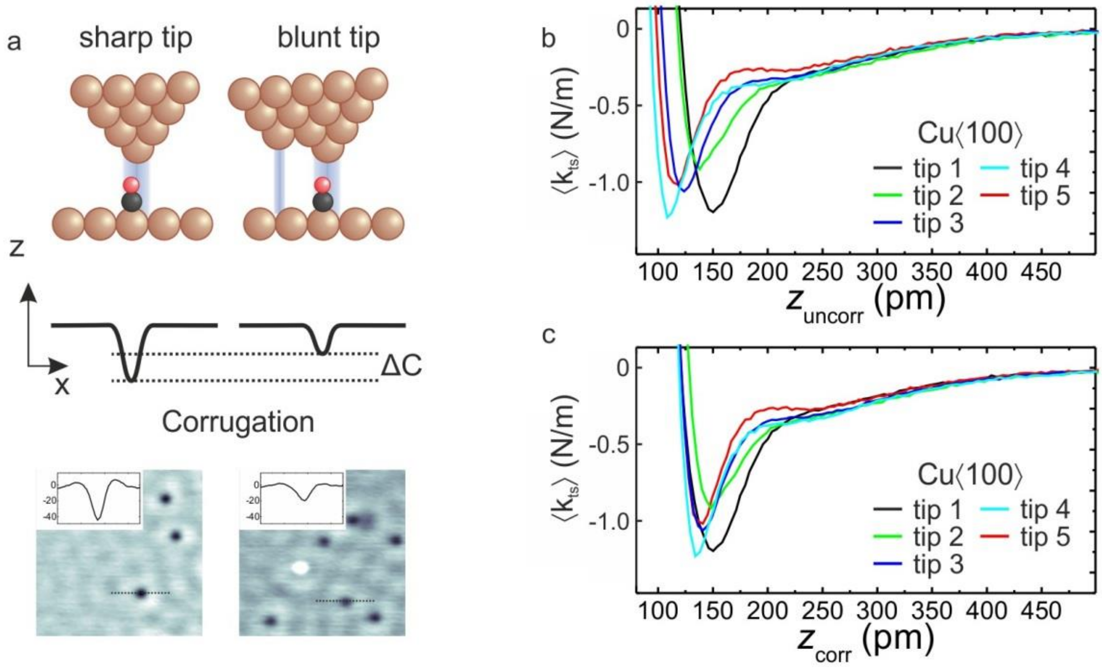


Fig. S 4 a) Illustration of the influence of a sharp compared to a blunt tip on the corrugation of the CO molecules. Parameters in the topography images: $I_{set}$ = 100 pA, $V_{sample}$ = - 10 mV. Blunt tips (i.e. tip 3 - 5) yield negative *z*-offsets in the uncorrected frequency shift-distance curves (b), while a sharp tip (tip 1) does not show a *z*-offset. This can be corrected by subtraction of $\Delta C$.

By combining equation (1) and (2), we find that the correct *z*-values can be calculated by the difference in the corrugations $\Delta C$ :

$$z_{corr} = z_{uncorr} + \Delta C \qquad (3)$$

Fig. S 4 displays a set of curves obtained with different Cu<100> tips before (b) and after the correction of the *z*-values (c), showing that the correction algorithm leads to less scattering in $<k_{ts}>(z)$ curves. The same correction algorithm is also used for all other tips, assuming that the topography image at large tip-sample distance is not influenced by the orientation and chemical nature of the tip.

## S 4 Variations in the force versus distance curves of Cu <100> tips due to various tip tilt angles

Fig. S 5 c shows the force versus distance curves of the three Cu <100> tips from Fig. 2 in the main text again. The position and the value of the force minimum as well as the shape of the force versus distance curves vary, although all curves are recorded with Cu tips oriented in the <100> direction. We conjecture that this variation is caused by slight variations of the tilt of the tip from a perfect <100> alignment. Fig. S 5 b displays profile curves through the COFI images (Fig. S 5 a) of the three tips. An asymmetry in the profiles is a measure for the tilt out of the <100> direction. We find that tip 1 shows the smallest tilt, while tip 2 is strongly tilted. Apparently, the tilt leads to a shift of the force minimum towards smaller *z* values. In addition, the valley around the force minimum becomes narrower and a shoulder develops at a *z* value of approximately 200 pm.

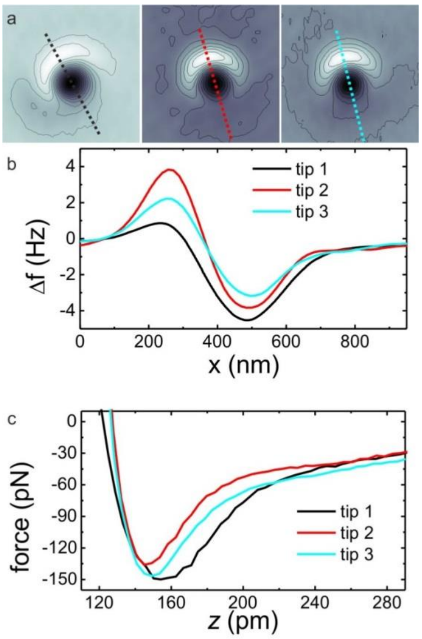


Fig. S 5 Influence of the tilt of Cu <100> tips on the shape of force versus distance curves: a) constant height frequency shift maps of tip 1, 2 and 3 with contour lines. b) Profile lines extracted from the COFI image at the position of the dotted lines (a). c) Force versus distance curves.

## S 5 Development of an electrostatic model that describes the orientation-dependent interaction of the Cu tip with the CO molecule

A simple electrostatic model was developed to explain the COFI images obtained with the Cu tips. With the help of the model the COFI images can be assigned to the three low-index high-symmetry directions of the Cu fcc crystal. In the following, the model is explained in detail.

First, we determine an electron distribution at the tip atom for the three highly symmetric tip clusters in Fig. S 6 b, namely the <100>, <111> and <110> orientations. We then calculate the electrostatic interaction force with the CO molecule, assuming a dipole moment of the CO molecule as proposed in Ref. [6].

The electronic states of the tip atom are approximated by atomic orbitals. We only consider the 3d orbitals because these show the directionality needed to explain the COFI images. All other orbitals are neglected. The 3d orbitals are described by Slater-type orbitals (STO) which have the following form (after [9], in SI units):

$$\Psi_{\mathrm{STO}}^{d_\mathrm{i}} = \sqrt{\frac{8}{45}}\chi^3 \frac{5}{a_\mathrm{B}^{1.5}} \frac{r^2}{a_\mathrm{B}^2} \exp\left(-\frac{\chi r}{a_\mathrm{B}}\right) \cdot d_\mathrm{i}, \quad (4)$$

where $r$ denotes the distance from the core, $a_\mathrm{B}$ is the Bohr radius and $d_\mathrm{i}$ is the spherical harmonic of the corresponding d orbital. The factor $\chi$ in the exponent determines the steepness of the wave function and is determined by the Slater rules [10]. We use a value of $\chi = 2.5$ which is slightly smaller than the value determined from the Slater rules to accommodate for the partial screening of the core charges by other electrons of neighboring tip atoms.

In an isolated neutral Cu atom, the 3d shell is completely filled. In a surface atom, and in particular in the case of an exposed front atom of a tip, the tip atom is positively charged due to the Smoluchowski effect. Additionally, the 3d orbitals are not equally occupied because they are affected

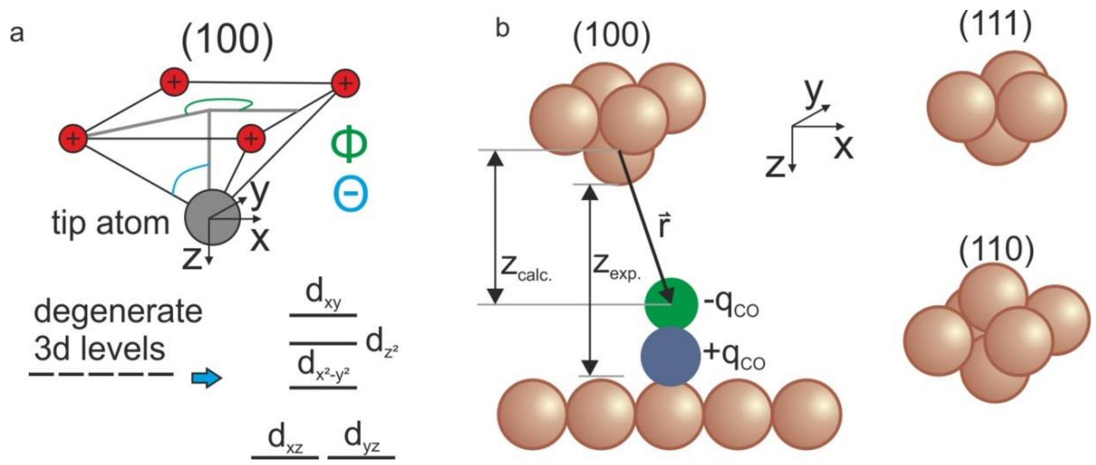


Fig. S 6 a) The crystal field of the nearest neighbors leads to a splitting of the energy levels of the 3d orbitals, as shown for the case of a Cu<110> tip. Angles $\theta$ and $\phi$ are used to calculate the overlap of each 3d orbital with the nearest neighbors. b) Tip atoms for the three tip clusters are modeled and their electrostatic interaction with the CO molecule is calculated. The origin of the coordinate system is in the center of the tip atom. The vertical height used in the calculation $z_\mathrm{calc}$ is set to the experimental value $z_\mathrm{exp}$ (see section S2).

by the partially unscreened cores of the nearest neighbors. According to crystal field theory [11] the energy levels of the 3d orbitals will split in this electric field, as illustrated in the example of a Cu<100> tip in Fig. S 6 a: An orbital which shows a large overlap with the positive charge of the nearest neighbors will be lower in energy compared to an orbital with small overlap. The relative energy splitting among the 3d orbitals is estimated with the help of the angular overlap model (AOM) [12]. In this model the overlap of an orbital with a nearest neighbor is approximated by the value of its spherical harmonic in the direction of the nearest neighbor, specified by the angles $\theta_i$ and $\phi_i$ (see Table 1). The overlap with the different nearest neighbors is computed by summing up their individual contributions. The number of nearest neighbors depends on the orientation of the tip cluster and is 3, 4 or 5 for the <111>, <100> or <110> directions, respectively. For example, the relative energy splitting *ES* for a Cu<100> tip is calculated with the following expressions:

$$
\begin{aligned}
d_{z^2} : ES_{d_{z^2}} &= 4\frac{1}{4}\left(3\cos(\theta_1) - 1\right)^2 S_\sigma^2 \\
d_{xz} : ES_{d_{xz}} &= 3\sin^2(\theta_1)\cos^2(\theta_1)\left[\cos^2(\phi_1) + \cos^2(\phi_2) + ..\right]S_\sigma^2 \\
d_{yz} : ES_{d_{yz}} &= 3\sin^2(\theta_1)\cos^2(\theta_1)\left[\sin^2(\phi_1) + \sin^2(\phi_2) + ..\right]S_\sigma^2 \\
d_{xy} : ES_{d_{xy}} &= 3\sin^4(\theta_1)\left[\sin^2(\phi_1)\cos^2(\phi_1) + \sin^2(\phi_2)\cos^2(\phi_2) + ..\right]S_\sigma^2 \\
d_{xz} : ES_{d_{xz}} &= \frac{3}{4}\sin^4(\theta_1)\left[\left(1 - 2\sin^2(\phi_1)\right)^2 + \left(1 - 2\sin^2(\phi_2)\right)^2 + ..\right]S_\sigma^2 .
\end{aligned}
\tag{5}
$$

The overlap factor $S_\sigma$ is arbitrarily set to 1. A high *ES* value corresponds to a low lying energy level. We use the normalized relative energy splitting $\alpha_i = ES_i/\sum_j ES_j$ to calculate an approximation for the occupation $q_{di}$ of the d orbitals. The d orbitals at the lowest energy level are assumed to be fully occupied with two electrons. The other orbitals are filled according to the normalized splitting energy:

$$q_{d_i} = 2e\frac{\alpha_i}{\max(\alpha_i)} \quad . \tag{6}$$

The charge density at the tip atom is then given by the sum of probability densities of the 3d orbitals times their occupation $q_{di}$:

$$\rho(\vec{r}) = \sum_i q_{d_i} \left|\Psi_{STO}^{d_i}(\vec{r})\right|^2 \quad . \tag{7}$$

The total negative charge of the tip atom is simply the sum over the occupation numbers $\sum_i q_{di}$. The total occupations of the 3d shell of the Cu tip atom are 5.33 e, 6 e and 6.65 e in the case of the

| Tip orientation | $\theta_i$ | $\phi_i$ |
|---|---|---|
| 100 | 45° | 0, 90°, 180°, 270° |
| 111 | 54,73° | 0, 120°, 240° |
| 110 | 60°, 0° | 35.26°, 144.74°, 215.26°, 324.74° |

Table 1: Angles $\theta_i$ and $\phi_i$ in the direction of the nearest-neighbors for the three orientations of the tip cluster: The angles are used to calculate the relative shift of the energy levels and hence the occupations of the five different 3d orbitals.

Cu<100>, Cu<111> and Cu<110> tips, respectively.

Fig. S 7 shows the electron densities $\rho(x,y,z)$ for the three tip atoms. In the case of the Cu<100> tip the electron density shows a torus in the *x-y* plane over the whole distance regime with a lower electron density in the center. For the Cu<111> tip the electron density has the shape of a two-dimensional gaussian for large *z* values. Close to the center of the atom, the charge density also becomes toroidal, although its diameter is smaller compared to the Cu<100> tip. The electron density at the tip atom of the Cu<110> is not symmetric with respect to rotations around the *z* axis for the whole distance regime. This asymmetry is strongly enhanced for small distances. In summary, we find that the symmetry found in the COFI images is already reflected in the projections of the electron density, especially for small *z* values.

In the next step, we calculate the interaction of the modeled electron density with the CO molecule. We assume that the interaction can be estimated by an electrostatic potential. For this purpose, the CO molecule is modeled as a dipole with a dipole moment of $p = q_{CO} \times h = 0.1$ e × 100 pm = = 0.48 Debye (a dipole moment of 0.123 e x 100 pm is calculated in Ref. [13] for CO/Cu) pointing away from the Cu tip (negative charge on the oxygen [13], see Fig. S 6 b). Therefore we obtain a repulsive force in regions of high electron density. Similar results are expected if the interaction was calculated by means of Pauli repulsion, as the magnitude of the repulsive force is also proportional to the electron density [14]. However, we clearly observe attractive interaction in some lateral positions and Pauli repulsion cannot fully explain the short range forces, while electrostatic interaction can.

In the electrostatic calculation the negative charge of the 3d orbitals is compensated with a positive charge in the center of the tip atom $Q_{\text{core}}$. By adjusting the magnitude of $Q_{\text{core}}$ we can tune the net charge of the front atom such that realistic values (less than one electronic charge) result in spite of the partial filling of the d shells. Adjusting $Q_{\text{core}}$ also allows to fit the force versus distance curve derived from the model potential to the experimental force curves (see Fig. 1 main text).

The model potential has the following form:

$V_{\text{tip-CO}} = V(x,y,z) - V(x,y,z+h)$ with $h$ = 100 pm (CO modelled as a dipole with charges +/- 0.1 e spaced by a distance of 100 pm) and

$$V(x,y,z) = \frac{q_{CO}}{4\pi\varepsilon_0}\left[\int_{x'=-\infty}^{\infty} dx' \int_{y'=-\infty}^{\infty} dy' \int_{z'=-\infty}^{\infty} dz' \frac{\sum_i q_{d_i} \left|\Psi_{\text{STO}}^{d_i}(x',y',z')\right|^2}{\sqrt{(x-x')^2+(y-y')^2+(z-z')^2}} - \frac{Q_{core}}{\sqrt{x^2+y^2+z^2}}\right]. \quad (8)$$

The best agreement between the model and the experimental data is obtained for core charges $Q_{\text{core}}$ = +5.58 e, +6.52 e and +6.69 e for the Cu<100>, Cu<111> and Cu<110> tips, respectively. As a result, the net charge of the tip atoms is positive for all three orientations with values of +0.25 e, +0.52 e and +0.04 e for the Cu<100>, Cu<111> and Cu<110> tips, respectively.

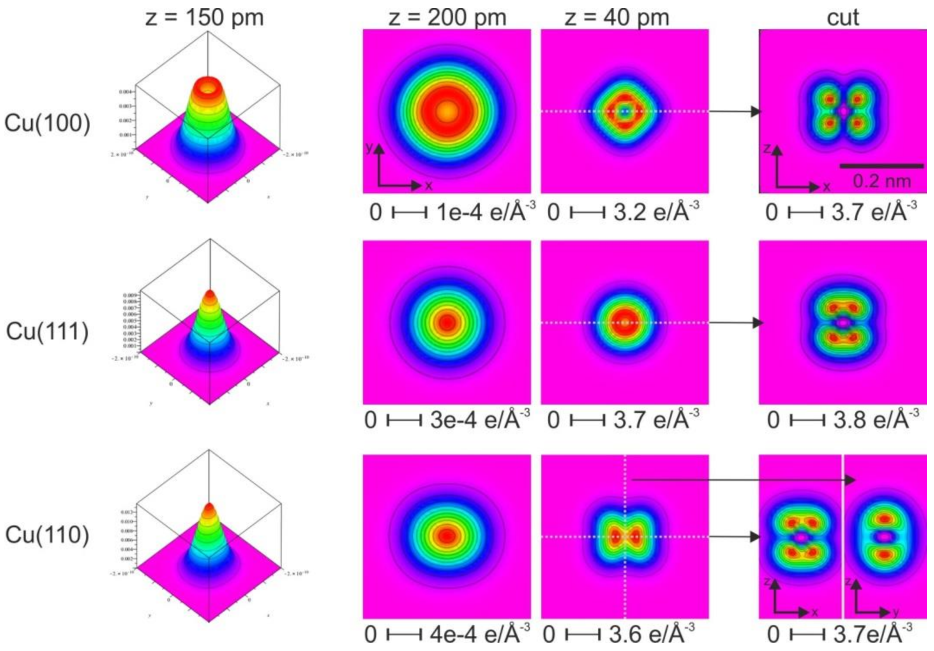


Fig. S 7 Calculated electron densities for tip atoms of Cu<100>, Cu<111> and Cu<110> tips. A 3D view and projections on the x-y and on the x-z plane (Cu<110> *x-z* and *y-z* planes) are shown. The size of the images is 400 × 400 pm$^2$ and the center of the tip atom is in the center of the picture (with exception of the *x-z*/*y-z* image of the Cu<110> tip).

It is important to comment on the total charge of the Cu front atom here. For an isolated Cu atom, the d shell is completely filled with 10 electrons, and in our model, it is only approximately half filled. However, the total charge is still well below one elementary charge. The validity of comparing electronic states of a free atom in vacuum to an atom in bulk is of course limited – the Coulomb potential of a free atom is perfectly rotationally symmetric, while the front atom of the tip is subject to an electric field that is strongly affected by the atomic neighbors. We still trust that using free-atom states is useful and instructive, and we conjecture that the remaining d electrons might go into bulk-like states that are only weakly dependent on rotations around the *z*-axis of the tip.

## S 6 Tip symmetries in the current image

In the CH current maps, which were acquired together with the $<k_{ts}>$ maps, we observe a dip over the CO molecule which has approximately the shape of a cylindrical Gaussian function (Fig. S 8). However, the non-cylindrical patterns observed in the frequency shift images that mark the tip symmetries involve lateral forces, which in turn affect the shape of the current dips. The reason is that the CO molecule is bent in the force field of the tip atom, as discussed in detail in Fig. 3 and supplemental material of Ref [6]. This leads to a variation of the current minimum, as explained in Ref. [6]. We can make this variation visible by applying a Laplace filter to the current. In Fig. S 8 the result is shown for all three orientations of the Cu tip atoms. The filtered current images reveal similar features like the frequency shift maps. However, no clear difference can be observed between the Cu<100> and the Cu<111> tip. Therefore it is not possible to distinguish them by STM. Nevertheless, it is important to note that features of tip symmetry can be observed by plain STM: recording constant height images (or even topographic images) over CO molecules adsorbed on Cu (111) at distances close to the manipulation distance reveals small variations in the current- or topographic images that show up after Laplace-filtering.

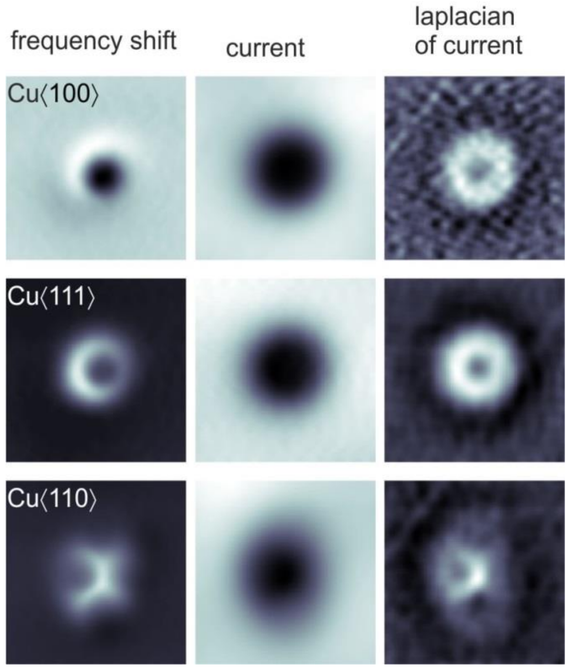


Fig. S 8: Average force gradient $<k_{ts}>$ and current maps together with the images of the Laplace filtered current maps of the three high symmetry Cu tips.

## S 7 Additional examples of COFI images of various Cu tips

Fig. S 9 shows the effect of the tilt of the tip cluster on the appearance of COFI images. Because of the random nature of tip pokes, perfect alignment in a high-symmetry direction is never achieved. However, the deviations from a perfect alignment can become small after a sufficient number of pokes (see also Fig. S 9 in Ref. [6]).

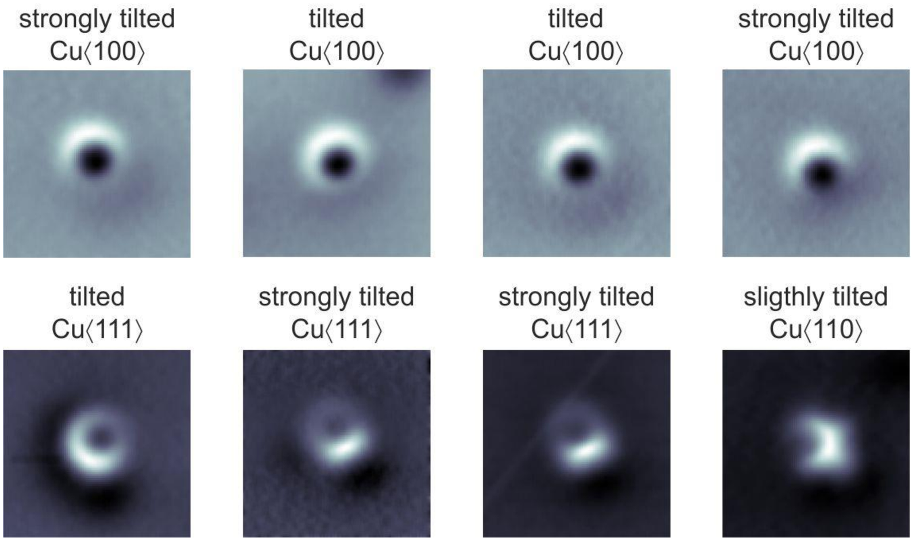


Fig. S 9 Additional examples of COFI images of various Cu tips with various tilt angles. Scan sizes are $1.5 \times 1.5$ nm$^2$ for all images.

## S 8 Threefold symmetries in bcc tips (Fe, W)

The highest angular momentum states of d orbitals yield a twofold symmetry with respect to rotations around the *z*-axis. A threefold symmetry with respect to the *z* axis requires f orbitals. However, it is possible to create states from d orbitals that are threefold symmetric with respect to a <111> axis. A linear combination of $d_{xz}$, $d_{yz}$ and $d_{xy}$ orbitals with equal weights creates a charge density proportional to $(x^2z^2 + y^2z^2 + x^2y^2)$. Such a charge density has local maxima in the <111> directions, i.e. along the nearest neighbor directions in bcc crystals such as W and Fe, and this charge density is threefold symmetric with respect to rotations around the <111> axes.

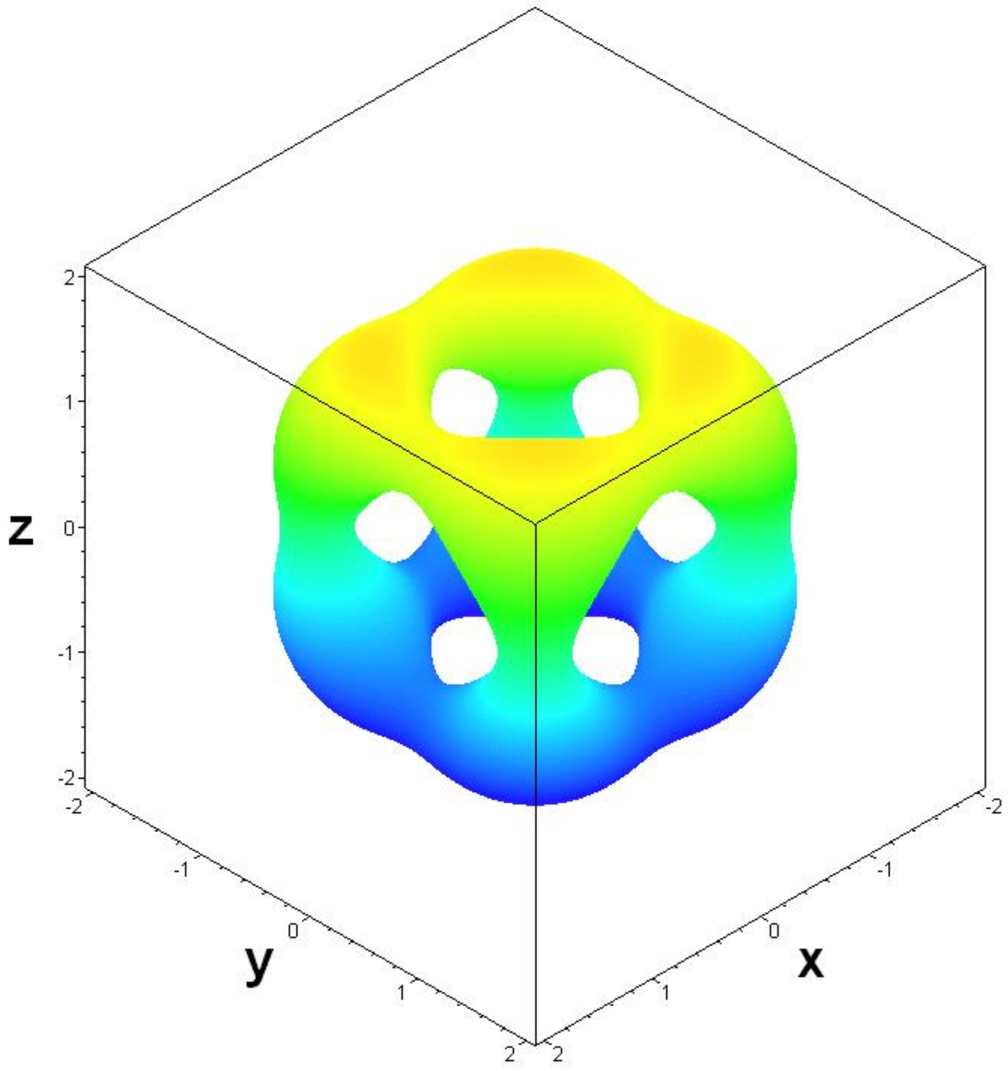


Fig. S 10 Schematic charge-density plot for a bcc tip with equally occupied $d_{xz}$, $d_{yz}$ and $d_{xy}$ states and empty $d_{x^2-y^2}$ and $d_{z^2}$ states, yielding a charge density that is threefold symmetric with respect to rotations around a <111> axis.

References:

[1] E. Müller and K. Bahadur, Phys. Rev. **102**, 624 (1956).

[2] L. Limot, J. Kröger, R. Berndt, A. Garcia-Lekue, and W. A. Hofer, Phys. Rev. Lett. **94**, 126102 (2005).

[3] G. Schull, T. Frederiksen, A. Arnau, D. Sánchez-Portal, and R. Berndt, Nat. Nanotechnol. **6**, 23 (2011).

[4] F. Mohn, B. Schuler, L. Gross, and G. Meyer, Appl. Phys. Lett. **102**, 073109 (2013).

[5] S.-W. Hla, K.-F. Braun, V. Iancu, and A. Deshpande, Nano Lett. **4**, 1997 (2004).

[6] J. Welker and F. J. Giessibl, Science **336**, 444 (2012).

[7] M. Ternes, C. González, C. P. Lutz, P. Hapala, F. J. Giessibl, P. Jelínek, and A. J. Heinrich, Phys. Rev. Lett. **106**, 016802 (2011).

[8] J. E. Sader and S. P. Jarvis, Appl. Phys. Lett. **84**, 1801 (2004).

[9] R. McWeeny, *Coulson`s Valence*, 3rd Edition (Oxford University Press, Oxford, 1979).

[10] J. Slater, Phys. Rev. **36**, 57 (1930).

[11] J. Van Vleck, Phys. Rev. **41**, 208 (1932).

[12] C. E. Schäffer and C. K. Jørgensen, Mol. Phys. **9**, 401 (1965).

[13] M. Feng, P. Cabrera-Sanfelix, C. Lin, A. Arnau, D. Sánchez-Portal, J. Zhao, P. M. Echenique, and H. Petek, ACS Nano **5**, 8877 (2011).

[14] N. Moll, L. Gross, F. Mohn, A. Curioni, and G. Meyer, New J. Phys. **14**, 083023 (2012).
